# Supplementary material for: Time Waits for No One! Analysis and Challenges of Temporal Misalignment
Source: arXiv:2111.07408 source file (2022-07-01)
Supplement: Supplementary file 1 [file appendix.tex]

\begin{figure*}[]
    \centering
\includegraphics[width=0.9\textwidth]{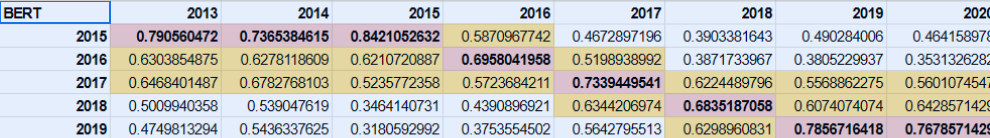}
\caption{Political party prediction based on tweets (BERT).}
\label{table:bert_twitter_downstream}
\end{figure*}
